# Supplementary material for: BRIGHT: A Realistic and Challenging Benchmark for Reasoning-Intensive Retrieval
Source: arXiv:2407.12883 source file (2025-03-26)
Supplement: Supplementary file 1 [file case_study.tex]

\section{Case Study: Retrieving Relevant Examples Improves Model Performance}
\label{sec:case_study}
\ours is designed to meet users' needs to retrieve documents that are intrinsically relevant to the query beyond simple semantic matching. Besides serving users with retrieved documents, these documents can also be used as context for language models to provide an answer to the query directly, known as retrieval augmented generation (RAG). While our work focuses on evaluating retrieval performance, we also provide a case study in the RAG setting. This illustrates how annotated documents from \ours can enhance the performance of language models to solve the query, whereas documents retrieved from state-of-the-art retrieval systems fail to do so. 

We present an example from the \theorem dataset, where the query is a math problem that essentially requires using an integral rule to derive the original form of the function. 
Our gold positive example features a similar problem utilizing the same theorem. 
With this gold example as context, our model---\ttt{gpt-4-0125-preview}---successfully derives the correct solution, despite the surface differences between the gold positive example and the query. 
In contrast, the random example and the examples retrieved by BM25 and Qwen do not require the use of the integral rule; instead, they feature algebraic and combinatoric problems, respectively. 
With the retrieved example in the context, the model fails to derive the correct solution. 
This case study demonstrates that our gold annotation also has the potential to improve RAG performance by providing relevant examples. 
We will leave a systematic evaluation of RAG for future work.

\begin{example}[Query (a math problem from \theorem)]
\begin{lstlisting}
You're tracking the growth of a plant from a seed. The rate at which 
the plant grows in height is equal to the square root of the number 
of days since you planted it. One day after the seed was first 
planted, the plant was 1 inch tall. How tall will the plant be after 
4 days?
  \end{lstlisting}
\end{example}
\begin{correctanswer}
\small{\textbf{Gold Positive Example}: 
  ${\frac{dy}{dx}} = \sqrt{t}, y(1) = 1$. What is $y(16)$?\newline\newline
  To find $y(4)$, we need to solve the given differential equation and apply the initial condition $y(1) = 1$.\newline
  The given differential equation is: ${\frac{dy}{dx}} = \sqrt{t}$\newline
  To solve this, we can integrate both sides with respect to $t$:\newline
  $\int dy = \int \sqrt{t} \, dt$\newline
  $y(t) = (2/3)t^{(3/2)} + C$ \newline
  Now, we apply the initial condition $y(1) = 1$: \newline
  $1 = (2/3)(1)^{(3/2)} + C$\newline
  $1 = 2/3 + C$\newline
  $C = 1/3$\newline
  So, the solution to the differential equation is: $y(t) = (2/3)t^{(3/2)} + 1/3$\newline
  Now, we can find $y(16)$:\newline
  $y(4) = (2/3)(16)^{(3/2)} + 1/3$\newline
  $y(4) = (2/3)(64) + 1/3$\newline
  $y(4) = 128/3 + 1/3$\newline
  $y(4) = 43$\newline
  Therefore, the answer is $43$.\newline
  }

  \small{\textbf{Model Output \cmark}: The growth rate of the plant is given by the differential equation $\frac{dy}{dx} = \sqrt{t}$, with the initial condition $y(1) = 1$, which is exactly the same as the differential equation problem described above. Therefore, the solution process and the final solution apply here as well. We found that $y(t) = (2/3)t^(3/2) + 1/3$. To find the height of the plant after 4 days, we substitute $t = 4$ into this equation.\newline
  $y(4) = (2/3)(4)^(3/2) + 1/3 = 17/3$\newline
  Therefore, the plant will be 17/3 inches tall after 4 days. }
\end{correctanswer}

\begin{wronganswer}
\label{fig:random_example}
\small{\textbf{Random Example}: What is the smallest positive integer that can be multiplied by 605 to make it a perfect square?Answer Choices: (A) 2 (B) 3 (C) 5 (D) 7 (E) 11\newline\newline
Let's reason about the multi-choice question.\newline
605 is multiplied by 5 gives 3025\newline
Its a square root of 55\newline
The answer is 5 -Option C\newline}

\textbf{Model Output \xmark}: \small{The growth rate of the plant is equal to the square root of the number of days since it was planted. After 4 days, the height of the plant will be equal to the square root of 4, which is 2. Therefore, the plant will be 2 inches tall after 4 days.}
\end{wronganswer}

\begin{wronganswer}
\small{\textbf{BM25 Example}: A basketball team has 12 players, including 5 guards and 7 forwards. How many different starting lineups can be formed that include 3 guards and 2 forwards?\newline\newline
To form a starting lineup with 3 guards and 2 forwards, we need to choose 3 guards from the 5 available guards and 2 forwards from the 7 available forwards. We can use the combination formula to calculate this:\newline
Number of ways to choose 3 guards from 5 $= C(5, 3) = 5! / (3! * (5-3)!) = 10$\newline
Number of ways to choose 2 forwards from 7 $= C(7, 2) = 7! / (2! * (7-2)!) = 21$\newline
Now, we multiply the number of ways to choose guards and forwards to get the total number of different starting lineups:\newline
Total starting lineups = 10 (ways to choose guards) * 21 (ways to choose forwards) = 210\newline
Therefore, the answer is 210.\newline
}

\textbf{Model Output \xmark}: \small{To find the height of the plant after 4 days, we use the given rate of growth: the square root of the number of days since the plant was planted. Since the height of the plant is equal to the square root of the number of days, we just substitute 4 days into the formula:\newline
Height after 4 days = sqrt(4) = 2 inches.\newline
Thus, the plant will be 2 inches tall after 4 days.
}
\end{wronganswer}

\begin{wronganswer}
\label{fig:qwen_example}
 \small{\textbf{Qwen Example}: A basketball team has 10 players, but only 5 can play at a time. In how many ways can the coach choose the 5 players who will play in the starting lineup?\newline\newline
To determine the number of ways the coach can choose the 5 players for the starting lineup, we can use the combination formula. The combination formula is:\newline
$C(n, k) = n! / (k!(n-k)!)$\newline
where n is the total number of players (10 in this case), k is the number of players to choose (5 in this case), and ! denotes the factorial function $(e.g., 5! = 5 × 4 × 3 × 2 × 1)$.\newline
So, we have:\newline
$C(10, 5) = 10! / (5!(10-5)!)$\newline
$C(10, 5) = 10! / (5!5!)$\newline
Now, let's calculate the factorials:
$10! = 10 × 9 × 8 × 7 × 6 × 5 × 4 × 3 × 2 × 1 = 3,628,800$\newline
$5! = 5 × 4 × 3 × 2 × 1 = 120$\newline}

\small{\textbf{Model Output \xmark}: To determine the height of the plant after 4 days, we use the given growth rate formula: the height of the plant is equal to the square root of the number of days since it was planted.\newline
On day 1, the plant is 1 inch tall, which is consistent with the formula since the square root of 1 is 1.\newline
To find out the height after 4 days, we substitute the number of days (4) into the square root formula:\newline
Height $ = \sqrt{\text{days}} = \sqrt{4}$\newline
The square root of 4 is 2.\newline
Thus, the plant will be 2 inches tall after 4 days.
}

\end{wronganswer}
