# Supplementary material for: BRIGHT: A Realistic and Challenging Benchmark for Reasoning-Intensive Retrieval
Source: arXiv:2407.12883 source file (2025-03-26)
Supplement: Supplementary file 2 [file misc.tex]

\section{Dataset Documentation}
BRIGHT is the first text retrieval benchmark that requires intensive reasoning to retrieve relevant documents. The queries are collected from diverse domains (StackExchange, LeetCode, and math competitions), all sourced from realistic human data. Experiments show that existing retrieval models perform poorly on BRIGHT, where the highest score is only 21 measured by nDCG@10. BRIGHT provides a good testbed for future retrieval research in more realistic and challenging settings.

\paragraph{Data Card Author(s)}
\begin{itemize}
    \item \textbf{Hongjin Su, HKU:} Owner
    \item \textbf{Howard Yen, Princeton:} Owner
    \item \textbf{Mengzhou Xia, Princeton:} Owner
    \item \textbf{Weijia Shi, UW:} Contributor
    \item \textbf{Niklas Muennighoff:} Contributor
    \item \textbf{Han-yu Wang, HKU:} Contributor
    \item \textbf{Haisu Liu, HKU:} Contributor
    \item \textbf{Quan Shi, Princeton:} Contributor
    \item \textbf{Zachary S. Siegel, Princeton:} Contributor
    \item \textbf{Michael Tang, Princeton:} Contributor
    \item \textbf{Ruoxi Sun, Google:} Contributor
    \item \textbf{Jinsung Yoon, Google:} Contributor
    \item \textbf{Sercan Ö. Arik, Google:} Contributor
    \item \textbf{Danqi Chen, Princeton:} Contributor
    \item \textbf{Tao Yu, HKU:} Contributor
\end{itemize}

\subsection{Authorship}

\subsubsection{Publishers}

\paragraph{Publishing Organization(s)}
The University of Hong Kong

\paragraph{Industry Type(s)}
\begin{itemize}
    \item Academic - Tech
\end{itemize}

\paragraph{Contact Detail(s)}
\begin{itemize}
    \item \textbf{Publishing POC:} N/A
    \item \textbf{Affiliation:} N/A
    \item \textbf{Contact:} N/A
    \item \textbf{Mailing List:} N/A
    \item \textbf{Website:} N/A
\end{itemize}

\subsubsection{Dataset Owners}

\paragraph{Team(s)}
Hongjin Su, Howard Yen, and Mengzhou Xia

\paragraph{Contact Detail(s)}
\begin{itemize}
    \item \textbf{Dataset Owner(s):} Hongjin Su, Howard Yen, and Mengzhou Xia
    \item \textbf{Affiliation:} The University of Hong Kong and Princeton University
    \item \textbf{Contact:} hjsu@cs.hku.hk, \{hyen, mengzhou\}@cs.princeton.edu
    \item \textbf{Group Email:} N/A
    \item \textbf{Website:} N/A
\end{itemize}

\paragraph{Author(s)}
\begin{itemize}
    \item Hongjin Su, PhD student, The University of Hong Kong
    \item Howard Yen, Masters student, Princeton University
    \item Mengzhou Xia, PhD student, Princeton University
\end{itemize}

\subsubsection{Funding Sources}

\paragraph{Institution(s)}
\begin{itemize}
    \item Princeton University
    \item Google Cloud AI Research
\end{itemize}

\paragraph{Funding or Grant Summary(ies)}
We thank the Princeton University and Google Cloud AI Research for supporting Nvidia GPUs to benchmark retrieval models on BRIGHT.

\subsection{Dataset Overview}

\subsubsection{Data Subject(s)}
\begin{itemize}
    \item Non-Sensitive Data about people
    \item Public data accessible to everyone
\end{itemize}

\subsubsection{Dataset Snapshot}

\begin{tabular}{|l|l|}
\hline
Category & Data \\
\hline
Size of Dataset & 607 MB \\
Number of Instances & 1322 \\
Number of Fields & 6 \\
Domains & 11 \\
\hline
\end{tabular}

\textbf{Above:} We collect 1322 diverse queries from realistic human data. Each example is annotated with the gold documents and the reasoning traces to find them.

\subsubsection{Content Description}
The datasets are collected from \href{https://stackexchange.com/}{StackExchange}, \href{https://arxiv.org/abs/2305.12524}{TheoremQA}, \href{https://leetcode.com/}{LeetCode}, and \href{https://artofproblemsolving.com/}{Math competition}.

\subsubsection{Descriptive Statistics}

\begin{tabular}{|l|l|l|l|l|l|}
\hline
Dataset & \# Q & \# D & \# D+ & Q.L. & D.L. \\
\hline
Biology & 103 & 57,364 & 3.6 & 83.6 & 115.2 \\
Earth Science & 118 & 122,388 & 7.7 & 132.4 & 113.3 \\
Economics & 103 & 50,221 & 8.0 & 120.2 & 181.5 \\
Psychology & 101 & 52,841 & 7.3 & 118.2 & 149.6 \\
Robotics & 101 & 62,198 & 5.5 & 120.6 & 818.9 \\
Stack Overflow & 117 & 101,100 & 7.0 & 704.5 & 478.3 \\
Sustainable Living & 108 & 60,732 & 5.6 & 108.0 & 148.5 \\
LeetCode & 142 & 413,932 & 1.8 & 483.1 & 497.5 \\
Pony & 112 & 7,894 & 22.5 & 98.3 & 102.6 \\
AoPS & 111 & 188,177 & 4.7 & 89.0 & 250.5 \\
TheoremQA & 206 & 188,177 & 3.2 & 117.1 & 250.5 \\
\hline
\end{tabular}

Data statistics of BRIGHT. For each dataset, we show the number of queries (\# Q) and documents (\# D), the average number of positive documents (\# D+) per example, the average length of queries (Q.L.) and documents (D.L., measured by the GPT-2 tokenizer).

\subsubsection{Sensitivity of Data}

\paragraph{Sensitivity Type(s)}
\begin{itemize}
    \item None
\end{itemize}

\paragraph{Field(s) with Sensitive Data}
\begin{itemize}
    \item None
\end{itemize}

\paragraph{Security and Privacy Handling}
We select academia-oriented domains and remove all user information in StackExchange data.

\paragraph{Risk Type(s)}
\begin{itemize}
    \item No Known Risks
\end{itemize}

\paragraph{Supplemental Link(s)}
\begin{itemize}
    \item None
\end{itemize}

\paragraph{Risk(s) and Mitigation(s)}
\begin{itemize}
    \item N/A
\end{itemize}

\subsubsection{Dataset Version and Maintenance}

\paragraph{Maintenance Status}
\textbf{Actively Maintained} - No new versions will be made available, but this dataset will be actively maintained, including but not limited to updates to the data.

\paragraph{Version Details}
\begin{itemize}
    \item \textbf{Current Version:} 1.0
    \item \textbf{Last Updated:} 06/2024
    \item \textbf{Release Date:} 06/2024
\end{itemize}

\paragraph{Maintenance Plan}
We will mainly use Github issues and HuggingFace communities to address any issues the users encounter in using the BRIGHT data.

\textbf{Versioning:} If new versions are released, it will become 1.1 or 2.0 depending on the update.

\textbf{Updates:} There may be updates in the future.

\textbf{Errors:} We will address the errors users encounter.

\textbf{Feedback:} Either by email, Github issue, or HuggingFace community, we welcome all feedback to make this benchmark better.

\paragraph{Next Planned Update(s)}
\begin{itemize}
    \item \textbf{Version affected:} N/A
    \item \textbf{Next data update:} N/A
    \item \textbf{Next version:} N/A
    \item \textbf{Next version update:} N/A
\end{itemize}

\paragraph{Expected Change(s)}
\textbf{Updates to Data:} N/A

\textbf{Updates to Dataset:} N/A

\subsection{Example of Data Points}

\subsubsection{Primary Data Modality}
\begin{itemize}
    \item Text Data
\end{itemize}

\subsubsection{Sampling of Data Points}
\href{https://huggingface.co/datasets/xlangai/BRIGHT/blob/main/data_examples.pdf}{Typical Data Points Link}

\subsubsection{Typical Data Point}
Summarize here. Include any criteria for typicality of data point.

\begin{lstlisting}[breaklines]
  "query": "Claim in article about why insects are attracted to light\nIn this
  article they are addressing the reason insects are attracted to light when they say\nHeat radiation as an attractive component is refuted by the effect of LED lighting, which supplies negligible infrared radiation yet still entraps vast numbers of insects.\nI don't see why attraction to LEDs shows they're not seeking heat. Could they for example be evolutionarily programmed to associate light with heat? So that even though they don't encounter heat near/on the LEDs they still 'expect' to?",
  "reasoning": "The question probes why insects are drawn to low-heat LED lights, challenging the idea that their attraction to light is heat-based. The document helps distinguish between heat attraction and evolved behaviors, shedding light on why insects might be attracted to LEDs despite their minimal heat.",
  "id": "0",
  "excluded_ids": [
    "N/A"
  ],
  "gold_ids_long": [
    "insects_attracted_to_light/Proximate_and_ultimate_causation.txt",
    "insects_attracted_to_light/Phototaxis.txt"
  ],
  "gold_ids": [
    "insects_attracted_to_light/Phototaxis_3.txt",
    "insects_attracted_to_light/Proximate_and_ultimate_causation_0.txt",
    "insects_attracted_to_light/Phototaxis_4.txt",
    "insects_attracted_to_light/Proximate_and_ultimate_causation_1.txt",
    "insects_attracted_to_light/Phototaxis_0.txt"
  ]
}
\end{lstlisting}

\subsection{Motivations \& Intentions}

\subsubsection{Motivations}

\paragraph{Purpose(s)}
\begin{itemize}
    \item Research
\end{itemize}

\paragraph{Domain(s) of Application}
\texttt{retrieval}

\paragraph{Motivating Factor(s)}
\begin{itemize}
    \item Existing retrieval benchmarks can be solved by lexical or semantic match
    \item Many realistic scenarios cannot be solved by such simple match
    \item To bridge this gap, we introduce BRIGHT to evaluate retrieval models in realistic settings where intensive reasoning is required
\end{itemize}

\subsubsection{Intended Use}

\paragraph{Dataset Use(s)}
\begin{itemize}
    \item Evaluate retrieval systems in realistic scenarios
\end{itemize}

\paragraph{Suitable Use Case(s)}
\textbf{Suitable Use Case:} Evaluate retrieval models

\paragraph{Unsuitable Use Case(s)}
\textbf{Unsuitable Use Case:} Train retrieval models

\paragraph{Research and Problem Space(s)}
We investigate new directions of retrieval, where the relevance between queries and documents goes beyond lexical and semantic similarities.

\paragraph{Citation Guidelines}
\textbf{Guidelines \& Steps:} Include citation when using BRIGHT

\textbf{BiBTeX:}
\begin{lstlisting}[breaklines]
    @inproceedings{BRIGHT,
  title={BRIGHT: A Realistic and Challenging Benchmark for Reasoning-Intensive Retrieval},
  author={Su, Hongjin and Yen, Howard and Xia, Mengzhou and Shi, Weijia and Muennighoff, Niklas and Wang, Han-yu and Liu, Haisu and Shi, Quan and Siegel, Zachary S and Tang, Michael and Sun, Ruoxi and Yoon, Jinsung and Arik, Sercan O and Chen, Danqi and Yu, Tao},
  year={2024},
}
\end{lstlisting}

\subsection{Access, Rentention, \& Wipeout}
\subsubsection{Access}
\paragraph{Access Type}
% scope: telescope
% info: Select \textbf{one}:
- External - Open Access

\paragraph{Documentation Link(s)}
% scope: periscope
% info: Provide links that describe documentation to access this dataset:
- Dataset Website URL: \url{https://huggingface.co/datasets/xlangai/BRIGHT}
- GitHub URL: \url{https://github.com/xlang-ai/BRIGHT}

\paragraph{Prerequisite(s)}
% scope: microscope
% info: Please describe any required training or prerequisites to access this dataset.
N/A

\paragraph{Policy Link(s)}
% scope: periscope
% info: Provide a link to the access policy:
- Direct download URL: \url{https://huggingface.co/datasets/xlangai/BRIGHT}

Code to download data:
\begin{verbatim}
from datasets import load_dataset
data = load_dataset('xlangai/BRIGHT', 'examples')['biology']
\end{verbatim}

\paragraph{Access Control List(s)}
% scope: microscope
% info: List and summarize any access control lists associated with this dataset. Include links where necessary. Use additional notes to capture any other information relevant to accessing the dataset.
N/A

\subsubsection{Retention}
Free retention

\subsubsection{Wipeout and Deletion}
We are not currently considering wiping out or deleting the data

\subsection{Provenance}
\subsubsection{Collection}
\paragraph{Method(s) Used}
% scope: telescope
% info: Select \textbf{all applicable} methods used to collect data:
- Data are collected by authors

\paragraph{Methodology Detail(s)}
% scope: periscope
% info: Provide a description of each collection method used. Use additional notes to capture any other relevant information or considerations. (Usage Note: Duplicate and complete the following for collection method type.)
\textbf{Collection Type}

\textbf{Source:} \url{https://stackexchange.com/}, \url{https://arxiv.org/abs/2305.12524}, \url{https://leetcode.com/} and \url{https://artofproblemsolving.com/}.

\textbf{Platform:} N/A

\textbf{Is this source considered sensitive or high-risk?} No

\textbf{Dates of Collection:} 2024.03 to 2024.05

\textbf{Primary modality of collection data:}

% Usage Note: Select one for this collection type.

- Text Data

\textbf{Update Frequency for collected data:}

% Usage Note: Select one for this collection type.

- Static

\textbf{Additional Links for this collection:}

N/A

\paragraph{Source Description(s)}
\begin{itemize}
\item \textbf{Source:} StackExchange is a popular question-answering platform where users ask questions and receive answers from the community. \href{https://sustainability.stackexchange.com/questions/4691/how-good-is-it-to-reuse-water-from-plant-pots}{One example} is
\begin{lstlisting} [breaklines]
How good is it to reuse water from plant pots?
I'm living in an apartment, and after I water my plants the water goes to plates below the pots. The pots are in a metallic structure above the plates, so I can take the plates to reuse the water (throwing it at the plants again).
This reuse seems beneficial, because I think I can get rid of mosquitoes that would reproduce in the stagnated water. And also some nutrients of the soil (as well as earthworms) can return to the vase.
Is there some negative points in doing that?
EDIT: I think I must add that I'm at 3 degrees of latitude, in a hot and humid tropical rainforest, where the precipitation used to be around 1700 mm. So I use lots of water everyday, more than once a day sometimes, so the reused water is a small fraction of the water used.
waterreuseplants
Share
Improve this question
Follow
edited Mar 17, 2016 at 15:27
asked Sep 3, 2015 at 18:39
Rodrigo's user avatar
Rodrigo
16311 silver badge 66 bronze badges
i think you mean "pots" if they have dirt in them. "vases" hold water and cur flowers. - Kate Gregory Mar 17, 2016 at 14:53
Add a comment
2 Answers
Sorted by:
Highest score (default)
7
In my experience plants suffer in the long term from accumulation of salts in the soil, so fresh water would be better than reusing the water. Even better would be to get hold of fresh rain water (tricky in an apartment though, unless perhaps you have a balcony that gets rained on) for watering them, as that won't contain the salts that tap water does.
More detail here.
Share
Improve this answer
Follow
\end{lstlisting}
\item \textbf{Source:} LeetCode is a popular coding platform for programmers to practice. One example is:
\begin{lstlisting} [breaklines]
5. Longest Palindromic Substring
Medium
Topics
Companies
Hint
Given a string s, return the longest palindromic substring in s.
Example 1:
Input: s = "babad"
Output: "bab"
Explanation: "aba" is also a valid answer.
Example 2:
Input: s = "cbbd"
Output: "bb"
Constraints:
1 <= s.length <= 1000
s consist of only digits and English letters.
\end{lstlisting}

\item \textbf{Source:} \begin{lstlisting} [breaklines] AoPS contains math competition questions. [One example] is:
Problem 1
What is the ones digit of 222,22 -222,222, -2,222,-222222 
A. 0
B. 2
C. 4
D. 6
E. 8      

Solution 1
We can rewrite the expression as 222,222-(22,222+2,222+222+22+2).
We note that the units digit of the addition is 0 because all the units digits of the five numbers are 2 and 5*2=10, which has a units digit of 0.
Now, we have something with a units digit of 0 subtracted from 222,222. The units digit of this expression is obviously 2, and we get \boxed{B} as our answer.
\end{lstlisting}
\end{itemize}

\paragraph{Collection Cadence}
% scope: telescope
% info: Select \textbf{all applicable}:
\begin{itemize}
\item \textbf{Static:} Data was collected once from single or multiple sources.
\end{itemize}

\paragraph{Data Integration}
\begin{itemize}
\item \textbf{Source} N/A

\item \textbf{Included Fields} Data fields that were collected and are included in the dataset.

\begin{tabular}{|l|l|}
\hline
Field Name & Description \\
\hline
Post & The content of post where users ask questions \\
\hline
\end{tabular}

\item  \textbf{Additional Notes:} Add here

\item  \textbf{Excluded Fields} Data fields that were collected but are excluded from the dataset.

\begin{tabular}{|l|l|}
\hline
Field Name & Description \\
\hline
Answer & Community answers \\
Votes & The votes for the post of answers \\
\hline
\end{tabular}
\end{itemize}

\paragraph{Data Processing}
% scope: microscope
% info: Summarize how data from different sources or methods aggregated, processed, or connected. Use additional notes to capture any other relevant information or considerations. (Usage Note: Duplicate and complete the following for each source OR collection method.)

All the data collection and processing are done manually or with the help of python scripts.

\subsubsection{Collection Criteria}
\paragraph{Data Selection}
% scope: telescope
% info: Summarize the data selection criteria. Use additional notes to capture any other relevant information or considerations.
\begin{itemize}
\item \textbf{StackExchange:} We select posts that have links in answers receiving user accept or more than 5 votes
\item  \textbf{Math and Code:} We select questions that require a theorems of syntax documentation.
\end{itemize}

\paragraph{Data Inclusion}
% scope: periscope
% info: Summarize the data inclusion criteria. Use additional notes to capture any other relevant information or considerations.
We include data from diverse domains including psychology, robotics, etc.

\paragraph{Data Exclusion}
% scope: microscope
% info: Summarize the data exclusion criteria. Use additional notes to capture any other relevant information or considerations.
We exclude examples that do not require reasoning in retrieval or do not use theorems.

\subsubsection{Relationship to Source}
\paragraph{Use \& Utility(ies)}
% scope: telescope
% info: Describe how the resulting dataset is aligned with the purposes, motivations, or intended use of the upstream source(s). Use additional notes to capture any other relevant information or considerations. (Usage Note: Duplicate and complete the following for each source type.)
\begin{itemize}
\item \textbf{StackExchange:} We use the post and linked web pages in answers
\item \textbf{Math \& Code:} We use the questions and tags in websites.
\end{itemize}

\paragraph{Benefit and Value(s)}
% scope: periscope
% info: Summarize the benefits of the resulting dataset to its consumers, compared to the upstream source(s). Use additional notes to capture any other relevant information or considerations. (Usage Note: Duplicate and complete the following for each source type.)
- Using this method, we collect retrieval instances that require intensive reasoning to retrieve documents

\paragraph{Limitation(s) and Trade-Off(s)}
% scope: microscope
% info: What are the limitations of the resulting dataset to its consumers, compared to the upstream source(s)? Break down by source type. (Usage Note: Duplicate and complete the following for each source type.)
- The judgement of relevance can be subjective, leading to non-perfect human performance.

\subsubsection{Version and Maintenance}
% info: Fill this next row if this is not the first version of the dataset, and there is no data card available for the first version
\paragraph{First Version}
% scope: periscope
% info: Provide a \textbf{basic description of the first version} of this dataset.
- \textbf{Release date:} 06/2024
- \textbf{Link to dataset:} BRIGHT 1.0: \url{https://huggingface.co/datasets/xlangai/BRIGHT}
- \textbf{Status:} Actively Maintained
- \textbf{Size of Dataset:} 607 MB
- \textbf{Number of Instances:} 1322

\paragraph{Note(s) and Caveat(s)}
% scope: microscope
% info: Summarize the caveats or nuances of the first version of this dataset that may affect the use of the current version. Use additional notes to capture any other relevant information or considerations.
None

\paragraph{Cadence}
% scope: telescope
% info: Select \textbf{one}:
- Daily

\paragraph{Last and Next Update(s)}
% scope: periscope
% info: Please describe the update schedule:
- We have not updated the datasets since release.

\paragraph{Changes on Update(s)}
% scope: microscope
% info: Summarize the changes that occur when the dataset is refreshed. Use additional notes to capture any other relevant information or considerations. (Usage Note: Duplicate and complete the following for each source type.)
N/A

\subsection{Human and Other Sensitive Attributes}

\paragraph{Sensitive Human Attribute(s)}
None

\paragraph{Intentionality}
\begin{itemize}
\item \textbf{Intentionally Collected Attributes}
We only use human-labeled links or tags to find examples or documents, but not directly include human labels.

\item \textbf{Unintentionally Collected Attributes}
None

\end{itemize}

\paragraph{Rationale}
We follow links or tags to find relevant documents or examples.

\paragraph{Source(s)}
None

\paragraph{Methodology Detail(s)}
We follow links or tags to find relevant documents or examples.

\paragraph{Distribution(s)}
N/A

\paragraph{Known Correlations}
\begin{itemize}
    \item \textbf{Attributes:} \texttt{query}, \texttt{gold\_ids}, \texttt{gold\_ids\_long}
    \item \textbf{Description:} The documents corresponding to \texttt{gold\_ids} or \texttt{gold\_ids\_long} are relevant to queries.
    \item \textbf{Impact on dataset use:} It helps evaluate retrieval models in realistic setting.
\end{itemize}

\paragraph{Risk(s) and Mitigation(s)}
\begin{itemize}
\item \textbf{Human Attribute}
None
\end{itemize}

\subsection{Extended Use}

\subsubsection{Use with Other Data}

\paragraph{Safety Level}
\begin{itemize}
    \item Safe to use with other data
\end{itemize}

\paragraph{Known Safe Dataset(s) or Data Type(s)}
The data in BRIGHT benchmark focus on academia-oriented domains, and they should be safe.

\paragraph{Best Practices}
Evaluate retrieval systems on BRIGHT.

\paragraph{Known Unsafe Dataset(s) or Data Type(s)}
None

\paragraph{Limitation(s) and Recommendation(s)}
The judgement of relevance between queries and documents can be subjective, so marginal difference between model evaluation could be ignored, while significant difference gives good signals of model capabilities.

\subsubsection{Forking \& Sampling}

\paragraph{Safety Level}
\begin{itemize}
    \item Safe to form and/or sample
\end{itemize}

\paragraph{Acceptable Sampling Method(s)}
\begin{itemize}
    \item Cluster Sampling
    \item Haphazard Sampling
    \item Multi-stage sampling
    \item Random Sampling
    \item Retrospective Sampling
    \item Systematic Sampling
    \item Weighted Sampling
    \item Unsampled
\end{itemize}

\paragraph{Best Practice(s)}
Although sampling is possible, we recommend not to do it because the size of BRIGHT is not very large.

\paragraph{Risk(s) and Mitigation(s)}
N/A

\paragraph{Limitation(s) and Recommendation(s)}
N/A

\subsubsection{Use in ML or AI Systems}

\paragraph{Dataset Use(s)}
\begin{itemize}
    \item Evaluation
\end{itemize}

\paragraph{Notable Feature(s)}
The intensive reasoning required to retrieve documents.

\paragraph{Usage Guideline(s)}
\begin{itemize}
\item \textbf{Usage Guidelines:} Follow \href{https://github.com/xlang-ai/BRIGHT}{the tutorial} to evaluate retrieval systems.
\item \textbf{Approval Steps:} Steps are \href{https://github.com/xlang-ai/BRIGHT}{here}.

\item \textbf{Reviewer:} We authors review the dataset for publication.
\end{itemize}

\paragraph{Distribution(s)}
The BRIGHT benchmark is for the purpose of evaluation, i.e., all data are in test set.

\paragraph{Known Correlation(s)}
\begin{itemize}
    \item \textbf{Attributes:} \texttt{query}, \texttt{gold\_ids}, \texttt{gold\_ids\_long}
    \item \textbf{Description:} The documents corresponding to \texttt{gold\_ids} or \texttt{gold\_ids\_long} are relevant to queries.
    \item \textbf{Impact on dataset use:} It can help evaluate retrieval systems in more realistic scenarios.
    \item \textbf{Risks from correlation:} The judgement of correlation is by real users, and can be subjective.
\end{itemize}

\paragraph{Split Statistics}
\begin{itemize}
\item Data statistics of \ours
\\\\
\begin{tabular}{lcccccc}
\hline
\textbf{Dataset} & \textbf{\# Q} & \textbf{\# D} & \textbf{\# D+} & \textbf{Q.L.} & \textbf{D.L.} \\ \hline
Biology & 103 & 57,364 & 3.6 & 83.6 & 115.2 \\
Earth Science & 118 & 122,388 & 7.7 & 132.4 & 113.3 \\
Economics & 103 & 50,221 & 8.0 & 120.2 & 181.5 \\
Psychology & 101 & 52,841 & 7.3 & 118.2 & 149.6 \\
Robotics & 101 & 62,198 & 5.5 & 120.6 & 818.9 \\
Stack Overflow & 117 & 101,100 & 7.0 & 704.5 & 478.3 \\
Sustainable Living & 108 & 60,732 & 5.6 & 108.0 & 148.5 \\
LeetCode & 142 & 413,932 & 1.8 & 483.1 & 497.5 \\
Pony & 112 & 7,894 & 22.5 & 98.3 & 102.6 \\
AoPS & 111 & 188,177 & 4.7 & 89.0 & 250.5 \\
TheoremQA & 206 & 188,177 & 3.2 & 117.1 & 250.5 \\ \hline
\end{tabular}
\end{itemize}

For each dataset, we show the number of queries (\# Q) and documents (\# D), the average number of positive documents (\# D+) per example, the average length of queries (Q.L.) and documents (D.L., measured by the GPT-2 tokenizer).

\subsection{Transformations}
\textit{Fill this section if any transformations were applied in the creation of your dataset.}

\subsubsection{Synopsis}
\paragraph{Transformation(s) Applied}
\textit{Select all applicable transformations that were applied to the dataset.}
\begin{itemize}
    \item Data Aggregation
\end{itemize}

\paragraph{Field(s) Transformed}
\textit{Provide the fields in the dataset that were transformed. Use additional notes to capture any other relevant information or considerations.}
\begin{itemize}
    \item \textbf{Transformation Type}
    \begin{itemize}
        \item Field Name | Source \& Target \\
        gold\_ids | links: gold\_ids \\
        gold\_ids\_long | links: gold\_ids\_long
    \end{itemize}
\end{itemize}

\paragraph{Library(ies) and Method(s) Used}
\textit{Provide a description of the methods used to transform or process the dataset. Use additional notes to capture any other relevant information or considerations.}
\begin{itemize}
    \item \textbf{Transformation Type}
    \begin{itemize}
        \item \textbf{Method:} We follow the links or tags to find relevant documents.
        \item \textbf{Platforms, tools, or libraries:} We do not leverage other platforms or tools in transformation.
        \item \textbf{Transformation Results:} We collect 1322 examples that can be used for evaluating retrievers.
    \end{itemize}
\end{itemize}

\subsubsection{Breakdown of Transformations}
We find documents for all instances following the procedure above.

\paragraph{Residual \& Other Risk(s)}
\textit{What risks were introduced because of this transformation? Which risks were mitigated?}
The risk is that the relevance judgment is subjective.

\paragraph{Human Oversight Measure(s)}
\textit{What human oversight measures, including additional testing, investigations and approvals were taken due to this transformation?}
We require human annotators to write down the judgment for relevance and reasoning steps.

\paragraph{Additional Considerations}
\textit{What additional considerations were made?}
None

\paragraph{Cleaning Mismatched Value(s)}
We select high-quality data instances from websites, so there is no further cleaning.

\paragraph{Method(s) Used}
We follow links or tags on the websites.

\paragraph{Comparative Summary}
We do not use incorrect or mismatched values.

\paragraph{Residual \& Other Risk(s)}
N/A

\paragraph{Human Oversight Measure(s)}
The data and notes written down by annotators are reviewed.

\paragraph{Additional Considerations}
None

\paragraph{Anomalies}
We select data from websites, so no anomaly or outlier is excluded.

\paragraph{Method(s) Used}
N/A

\paragraph{Platforms, tools, or libraries:}
N/A

\paragraph{Comparative Summary}
N/A

\paragraph{Residual \& Other Risk(s)}
N/A

\paragraph{Human Oversight Measure(s)}
The data and notes written by annotators are reviewed.

\paragraph{Additional Considerations}
None

\paragraph{Dimensionality Reduction}
N/A

\paragraph{Method(s) Used}
N/A

\textbf{Platforms, tools, or libraries:}
N/A

\paragraph{Comparative Summary}
N/A

\paragraph{Residual \& Other Risks}
N/A

\paragraph{Human Oversight Measure(s)}
N/A

\paragraph{Additional Considerations}
None

\paragraph{Joining Input Sources}
We use StackExchange, LeetCode, TheoremQA, and math competitions.

\paragraph{Method(s) Used}
They are independent splits, so no join is performed.

\paragraph{Comparative Summary}
N/A

\paragraph{Residual \& Other Risk(s)}
N/A

\paragraph{Human Oversight Measure(s)}
N/A

\paragraph{Additional Considerations}
N/A

\paragraph{Redaction or Anonymization}
\textit{Which features were redacted or anonymized?}
N/A

\paragraph{Method(s) Used}
\textit{What methods were used to redact or anonymize data?}
N/A

\paragraph{Comparative Summary}
\textit{Why was data redacted or anonymized using this method over others? Provide comparative charts showing before and after redaction or anonymization process.}
N/A

\paragraph{Residual \& Other Risk(s)}
N/A

\paragraph{Human Oversight Measure(s)}
N/A

\paragraph{Additional Considerations}
N/A

\paragraph{Others (Please Specify)}
\textit{What was done? Which features or fields were affected?}
N/A

\paragraph{Method(s) Used}
N/A

\paragraph{Comparative Summary}
\textit{Why was this method used over others? Provide comparative charts showing before and after this transformation.}
N/A

\paragraph{Residual \& Other Risk(s)}
N/A

\paragraph{Human Oversight Measure(s)}
N/A

\paragraph{Additional Considerations}
N/A

\subsection{Annotations \& Labeling}
\paragraph{Annotation Workforce Type}
\begin{itemize}
    \item Human Annotations (Expert)
    \item Human Annotations (Non-Expert)
\end{itemize}

\paragraph{Annotation Characteristic(s)}
\begin{itemize}
    \item \textbf{Annotation Type} | \textbf{Number} \\
    Total number of annotations | 1322
\end{itemize}

\paragraph{Annotation Description(s)}
\textit{Provide descriptions of the annotations applied to the dataset. Include links and indicate platforms, tools or libraries used wherever possible. Use additional notes to capture any other relevant information or considerations.}
\begin{itemize}
    \item \textbf{Description:} Description of annotations (labels, ratings) produced. Include how this was created or authored. We follow links/tags to find relevant documents.
    \item \textbf{Link:} N/A
    \item \textbf{Platforms, tools, or libraries:} N/A
\end{itemize}

\paragraph{Annotation Distribution(s)}
\begin{itemize}
    \item \textbf{Dataset | number} \\
    Biology | 103 \\
    Earth Science | 118 \\
    Economics | 103 \\
    Psychology | 101 \\
    Robotics | 101 \\
    Stack Overflow | 117 \\
    Sustainable Living | 108 \\
    LeetCode | 142 \\
    Pony | 112 \\
    AoPS | 111 \\
    TheoremQA | 206
\end{itemize}
Distribution of data splits in each domain.

\paragraph{Annotation Task(s)}
    \begin{itemize}
        \item \textbf{Task description \& instructions:}
        In this section, we describe the instructions for annotators to collect data in BRIGHT.
        \begin{itemize}
            \item StackExchange
            \begin{itemize}
                \item Browse posts from the newest to the oldest.
                \item Discard posts without an answer accepted by the user or obtains more than 5 votes.
                \item Discard answers of posts without URL links.
                \item For each link in the answer, write down the answers to: (1) why are the document and the post relevant; (2) what is the reasoning required to understand the relevance between the post and the document. If these answers are not possible, discard the link.
                \item Use LLMs (e.g., ChatGPT, Claude, etc.) to generate post keywords, or use the post title to search for web pages with large keyword or semantic overlap in Google. Search for at most 5 negative web pages per query.
                \item Split every web page into small passages either by two newline symbols, "\#" in markdown files or fixed-length tokens.
            \end{itemize}
            \item TheoremQA
            \begin{itemize}
                \item In TheoremQA, the main task for the annotator is to check if the GPT-4 rewritten questions are valid.
                \item The specific instructions are as follows:
                \begin{itemize}
                    \item Read the rewritten question and determine if it is solvable.
                    \item If it is solvable, read the original question and solution, and determine if the rewritten question is consistent with the original question. That is, the same reasoning steps and the final answer should hold.
                    \item If it is also consistent, mark the question as valid, and make any minor edits to the problem statement (e.g., to improve grammar or fluency) as you see fit.
                    \item If it is not solvable or not consistent, read the original question and solution, and correct the rewritten question if possible. If not, then discard the problem.
                \end{itemize}
            \end{itemize}
            \item AoPS
            \begin{itemize}
                \item In AoPS, annotators are tasked to find questions from the AoPS Wiki and record the problems:
                \item Browse through the AoPS Wiki and find topic/category pages (example 1, example 2).
                \item Look through each page and find pages specific theorems or techniques that can be used to solve problems. The page should link to at least two competition problems (example 1, example 2).
                \item Record the links of both the theorem/technique as well as the problem pages.
                \item The annotators are assigned a category to look for theorems to avoid overlaps, and the categories are {algebra, geometry, calculus, probability, number theory, other}.
                \item After all links are collected, we use a web scraper to collect the problem statement and solutions, and we manually check the quality of the scraped data.
            \end{itemize}
            \item LeetCode
            \begin{itemize}
                \item In LeetCode, annotators determine whether a question is grounded in real-world concepts. We give a similar instruction to the annotator as to GPT-4:
                \begin{itemize}
                    \item Read the problem statement carefully.
                    \item Categorize the question into one of three categories: 0: The question is not grounded in any real-world concepts. The description only uses coding-specific terms, such as "linked list", "binary search", "palindrome", "sorting", etc., 1: The question is not grounded in any real-world concepts or real-world concepts that are commonly used in the context of coding, such as needle in a haystack, strings/words, or a spiral matrix.3, : The question is grounded in real-world concepts that are not commonly used in the context of coding, such as building height, planting trees, or games. It may still use some code-specific terms to specify the data structure involved.
                \end{itemize}
            \end{itemize}
        \end{itemize}
    \item \textbf{Methods used:} Basically, we follow links/tags to find documents.
    \item \textbf{Inter-rater adjudication policy:} Reviewers annotate where the pairing of queries and documents is not convincing.
    \item \textbf{Golden questions:} N/A
\end{itemize}

\subsubsection{Human Annotators}
\paragraph{Annotator Description(s)}
\begin{itemize}
    \item \textbf{Annotation Type}
    \begin{itemize}
        \item \textbf{Task type:} Annotate StackExchange data
        \item \textbf{Number of unique annotators:} 3
        \item \textbf{Expertise of annotators:} Both experts and non-experts
        \item \textbf{Description of annotators:} PhD students in computer science, biology, environment, etc.
        \item \textbf{Language distribution of annotators:} They all speak fluent English.
        \item \textbf{Geographic distribution of annotators:} They come from Asia.
        \item \textbf{Summary of annotation instructions:} Follow links to find documents with filtering.
        \item \textbf{Summary of gold questions:} N/A
        \item \textbf{Annotation platforms:} Google sheets
        \item \textbf{Additional Notes:} N/A
    \end{itemize}
\end{itemize}

\paragraph{Annotator Task(s)}
\begin{itemize}
    \item \textbf{Task Type}
    \begin{itemize}
        \item \textbf{Task description:} Annotate math and code data
        \item \textbf{Task instructions:} Follow tags to find similar problems/questions
        \item \textbf{Methods used:} Follow tags annotated by websites
        \item \textbf{Inter-rater adjudication policy:} The data is reviewed.
        \item \textbf{Golden questions:} N/A
        \item \textbf{Additional notes:} N/A
    \end{itemize}
\end{itemize}

\paragraph{Language(s)}
\begin{itemize}
    \item \textbf{Annotation Type}
    \begin{itemize}
        \item 100\% English
    \end{itemize}
\end{itemize}

\paragraph{Location(s)}
\begin{itemize}
    \item \textbf{Annotation Type}
    \begin{itemize}
        \item Asia [50 \%]
        \item US [50 \%]
    \end{itemize}
\end{itemize}

\paragraph{Gender(s)}
\begin{itemize}
    \item \textbf{Annotation Type}
    \begin{itemize}
        \item Male [80 \%]
        \item Female [20 \%]
    \end{itemize}
\end{itemize}

\subsection{Validation Types}
\subsubsection{Method(s)}
\textit{Select all applicable:}
\begin{itemize}
    \item Code/cross-reference Validation
\end{itemize}

\subsubsection{Breakdown(s)}
\begin{itemize}
    \item \textbf{Validation Type}
    \begin{itemize}
        \item \textbf{Number of Data Points Validated:} 1322
        \item \textbf{Fields Validated:} All fields in data are validated.
    \end{itemize}
\end{itemize}

\paragraph{Description(s)}
\begin{itemize}
    \item \textbf{Validation Type}
    \begin{itemize}
        \item \textbf{Method:} Describe the validation method here. Include links where necessary. We require annotators to write the logic to determine the relevance between queries and documents. The reviewers not only check the data, but also annotators' notes.
        \item \textbf{Validation Results:} Over 90\% of annotation passes peer review, and we discard the rest.
    \end{itemize}
\end{itemize}

\subsubsection{Description of Human Validators}
\paragraph{Characteristic(s)}
\textit{Provide characteristics of the validator pool(s). Use additional notes to capture any other relevant information or considerations.}
\begin{itemize}
    \item \textbf{Validation Type}
    \begin{itemize}
        \item Unique validators: 8
        \item Number of examples per validator: 300
        \item Average cost/task/validator: N/A
        \item Training provided: N
        \item Expertise required: N
    \end{itemize}
\end{itemize}

\paragraph{Description(s)}
\begin{itemize}
    \item \textbf{Validation Type}
    \begin{itemize}
        \item \textbf{Validator description:} Validators are domain experts, e.g., PhD students from the corresponding domains.
        \item \textbf{Training provided:} We do not provide training, but verify that the annotators, reviewers are qualified.
        \item \textbf{Validator selection criteria:} We have a test containing verified examples. An annotator is qualified if they can work out these examples.
        \item \textbf{Training provided:} N/A
    \end{itemize}
\end{itemize}

\paragraph{Language(s)}
\begin{itemize}
    \item \textbf{Validation Type}
    \begin{itemize}
        \item English [100 \%]
    \end{itemize}
\end{itemize}

\paragraph{Location(s)}
\begin{itemize}
    \item \textbf{Validation Type}
    \begin{itemize}
        \item Asia [60 \%]
        \item US [40 \%]
    \end{itemize}
\end{itemize}

\paragraph{Gender(s)}
\begin{itemize}
    \item \textbf{Validation Type}
    \begin{itemize}
        \item Male [70 \%]
        \item Female [30 \%]
    \end{itemize}
\end{itemize}

\subsection{Sampling Methods}
\subsubsection{Method(s) Used}
\textit{Select all applicable methods used in the creation of this dataset:}
\begin{itemize}
    \item Unsampled
\end{itemize}

\subsubsection{Characteristic(s)}
N/A

\subsubsection{Sampling Criteria}
N/A

\subsection{Known Applications \& Benchmarks}
\subsubsection{ML Application(s)}
\textit{Provide a list of key ML tasks that the dataset has been used for.}
\textit{Usage Note: Use comma-separated keywords.}
Retrieval evaluation

\subsubsection{Evaluation Result(s)}
\begin{itemize}
    \item SFR-Embedding-Mistral 17.8
    \item \textbf{Model Card:} \url{https://huggingface.co/Salesforce/SFR-Embedding-Mistral/tree/main}
    \item \textbf{Evaluation Results:}
    \begin{itemize}
        \item nDCG@10: 17.8
    \end{itemize}
\end{itemize}

\subsubsection{Evaluation Process(es)}
We write python scripts to run retrieval models on BRIGHT.

\paragraph{Description(s) and Statistic(s)}
\begin{itemize}
    \item SFR-Embedding-Mistral
    \begin{itemize}
        \item \textbf{Model Card:} \url{https://huggingface.co/Salesforce/SFR-Embedding-Mistral/tree/main}
        \item \textbf{Model Description:} The best-class retrieval model trained from mistral-7b.
        \begin{itemize}
            \item Model Size: 7.11B
            \item Model Weights: 7.11B
            \item Model Layers: 32
            \item Latency: 2s
        \end{itemize}
    \end{itemize}
\end{itemize}

\subsubsection{Expected Performance and Known Caveats}
\begin{itemize}
    \item Claude-3 + BM25
    \begin{itemize}
        \item \textbf{Expected Performance:} Surpasses results obtained without using LLMs.
        \item \textbf{Known Caveats:} The inference of LLMs can be expensive.
    \end{itemize}
\end{itemize}

\subsection{Terms of Art}
\subsubsection{Concepts and Definitions referenced in this Data Card}
\paragraph{BRIGHT}
\begin{itemize}
\item \textit{Definition: The name of this benchmark}
\item \textit{Source:}\url{https://huggingface.co/datasets/xlangai/BRIGHT}
\item \textit{Interpretation: N/A}
\end{itemize}

\subsection{Reflections on Data}
We believe that BRIGHT paves the way for future research on retrieval systems in more realistic and challenging settings.

\section{Other Dataset Information}
\subsection{Dataset URLs}
\textbf{URL to benchmark.} The benchmark URL can be found here: \href{https://huggingface.co/datasets/xlangai/BRIGHT}{link}

\textbf{URL to Croissant metadata.} The Croissant metadata URL can be found here: \href{https://huggingface.co/api/datasets/xlangai/BRIGHT/croissant}{link}

\subsection{Author Statement \& License Information}
 We the authors bear all responsibility in case of violation of rights. We provide the license information for the data we used to construct \ours{}:
 
 \textbf{StackExchange.} The data is publicly available and licensed under Creative Commons Attribution-ShareAlike license as follows:
\begin{itemize}
    \item Content contributed before 2011-04-08 (UTC) is distributed under the terms of CC BY-SA 2.5.
    \item Content contributed from 2011-04-08 up to but not including 2018-05-02 (UTC) is distributed under the terms of CC BY-SA 3.0.
    \item Content contributed on or after 2018-05-02 (UTC) is distributed under the terms of CC BY-SA 4.0.
\end{itemize}
Please find detailed information on the license at \url{https://stats.stackexchange.com/help/licensing}.

\textbf{LeetCode.} According to LeetCode's \href{https://leetcode.com/terms/}{Terms of Service}, the data on the platform is owned by the LeetCode Service. Following \cite{hendrycks2021measuring} and \cite{jain2024livecodebench}, we scrape the problem statement, solutions, test cases, similar problem annotations, and topics from the LeetCode website. We do not store any user data or any other proprietary information from the LeetCode platform. We abide by Fair Use §107: “the fair use of a copyrighted work, including such use by ... scholarship, or research, is not an infringement of copyright”, where fair use is determined by “the purpose and character of the use, including whether such use is of a commercial nature or is for nonprofit educational purposes” and “the effect of the use upon the potential market
for or value of the copyrighted work.”

\textbf{Pony.} Pony is licensed under apache-2.0 License according to its \href{https://huggingface.co/datasets/xlangai/arks_data}{HuggingFace dataset card}.

\textbf{TheoremQA \& AoPS.} TheoremQA is licensed under MIT License according to its \href{https://huggingface.co/datasets/TIGER-Lab/TheoremQA}{HuggingFace dataset card}. AoPS does not provide license information according to its \href{https://artofproblemsolving.com/wiki/index.php/AoPS_Wiki:Copyright}{Copyright statement}. 

\subsection{Hosting and maintenance.} We have a dedicated GitHub page to host the leaderboard (\url{https://brightbenchmark.github.io/}) while data and codebase will be hosted on Huggingface (\url{https://huggingface.co/datasets/xlangai/BRIGHT}) and GitHub (\url{https://github.com/xlang-ai/bright}). We are committed to performing major maintenance on \ours{} every 3-6 months.
